# Supplementary material for: Gapless Dirac magnons in CrCl$_{3}$
Source: arXiv:2110.10771 source file (2021-10-20)
Supplement: Supplementary file 1 [file CrCl3Supplement.pdf]

# Supplemental Materials: Gapless Dirac magnons in $CrCl_3$

John A. Schneeloch,[1] Yu Tao,[1] Yongqiang Cheng,[2] Luke Daemen,[2] Guangyong Xu,[3] Qiang Zhang,[2] and Despina Louca[1,*]

[1]*Department of Physics, University of Virginia, Charlottesville, Virginia 22904, USA*
[2]*Neutron Scattering Division, Oak Ridge National Laboratory, Oak Ridge, Tennessee 37831, USA*
[3]*NIST Center for Neutron Research, National Institute of Standards and Technology, Gaithersburg, Maryland 20877, USA*

## EFFECT OF STACKING DISORDER ON $(300)_R$ POSITION

In this section, we argue that Bragg peaks $(H, K, 0)_R$ with $H$ and $K$ divisible by 3 are largely immune to stacking disorder, and that the relative difference in position between equivalent peaks in the $R\bar{3}$ and $C2/m$ phases are expected to be $\sim 2 \cdot 10^{-5}$ and thus much less than the observed lattice constant anomaly ($\sim 6 \cdot 10^{-4}$).

We assume that the intralayer structure of $CrCl_3$ is unchanged aside from overall changes in the lattice parameters. We assume that, although the trigonal symmetry of a layer is broken in the $C2/m$ phase, we still have $b_M = \sqrt{3} a_M$, which holds true within uncertainty according to reported coordinates [1].

The structure factor of a Bragg peak in elastic neutron scattering is given by:

$$F = \sum_j b_j e^{i\mathbf{G}\cdot\mathbf{d}_j} \tag{1}$$

where the $j$ index sums over every atom in the unit cell (which have nuclear scattering lengths $b_j$ and positions $\mathbf{d}_j$), and $\mathbf{G}$ is the Bragg peak wavevector. (The Debye-Waller factor is presumed to be $\sim 1$ and is neglected.) A similar formula holds for X-ray diffraction, except with the $b_j$ replaced by $Q$-dependent atomic form factors. For arbitrary stacking, we can expand the unit cell in the out-of-plane direction to an arbitrary extent. If we let $F_0$ be the structure factor for a single layer, then the overall structure factor is:

$$F = \sum_n F_0 e^{i2\pi nL} e^{i2\pi(H_R s_{x,n} + K_R s_{y,n})} \tag{2}$$

where we use rhombohedral coordinates and where $(s_{x,n}, s_{y,n}, 0)_R$ is the overall in-plane translation of layer $n$ relative to layer 0.

For LT-type stacking, each layer has two possible in-plane translations relative to the layer below it: $\pm(1/3, 2/3, 0)_R$. Thus, if $H_R + 2K_R$ is divisible by 3, the structure factor remains the same regardless of the sequence of stacking choices. The $R\bar{3}$ phase is constructed by repeating one such choice indefinitely (3 times to construct the unit cell).

For HT-type stacking, each layer has three possible in-plane translations relative to the layer below it: $\alpha(1/3, 0, 0)_R$, $\alpha(0, 1/3, 0)_R$, or $\alpha(-1/3, -1/3, 0)_R$, where $\alpha \approx 0.978$ (i.e., close to unity) as determined from reported coordinates [1]. (Fundamentally, the LT- and HT-type stacking choices come from the two ways one can place the triangular lattices formed by a layer's $Cl^-$ ions on top of each other.) Thus, assuming $\alpha \approx 1$, requiring $H$ and $K$ each be divisible by 3 results in minimal change in Bragg peak intensity with HT-type stacking variation (and LT-type stacking as well, as discussed above.) Figure S1 shows an X-ray diffraction pattern in the $(H0L)_M$ scattering plane of a single crystal cooled from room temperature to 110 K. The transition into the $R\bar{3}$ phase was frustrated, resulting in stacking disorder that manifested as diffuse scattering streaks along the $L$-direction (similar to those reported for $\alpha$-$RuCl_3$ [2].) However, the peaks at $(\bar{6}0L)_M$ are undisturbed for the reasons discussed above. Likewise, from the neutron powder diffraction data seen in Fig. S2(a), the $(300)_R$ intensity is largely unchanged despite the onset of stacking disorder.

The $(300)_R$ Bragg peak overlaps with the $(060)_M$ and $(33\bar{1})$ Bragg peaks. While $(060)_M$ depends only on the in-plane lattice constants, $(33\bar{1})$ is not quite in the $(HK0)_R$ scattering plane since $\alpha \neq 1$. In detail, if we assume the in-plane lattice constants depend only on temperature (so $a_M = a_R$ if two phases coexist at a certain temperature), that $b_M = \sqrt{3} a_M$, and that $\alpha$ has the same value at low temperature as at high temperature, then we have

$$|\mathbf{Q}_{(300)_R}| = |\mathbf{Q}_{(060)_M}| = 2\sqrt{3}\frac{2\pi}{a} \tag{3}$$

and

$$\begin{aligned} |\mathbf{Q}_{(33\bar{1})_M}| &= \frac{2\pi}{V_M} 6as\sqrt{1 + \frac{a^2}{12s^2}(\alpha - 1)^2} \\ &\approx \frac{2\pi}{V_M} 6as(1 + \frac{a^2}{24s^2}(\alpha - 1)^2) \end{aligned} \tag{4}$$

where $s$ is the interlayer spacing $\sim 5.78$ Å. The expected relative difference in the position of $(33\bar{1})_M$ as compared to $(060)_M$ or $(300)_R$ is thus $\sim 2.1 \cdot 10^{-5}$.

## ADDITIONAL DATA

In this section, we show data on the lattice parameters measured at POWGEN and SPINS. In Fig. S3(a), the

* Corresponding author; louca@virginia.edu

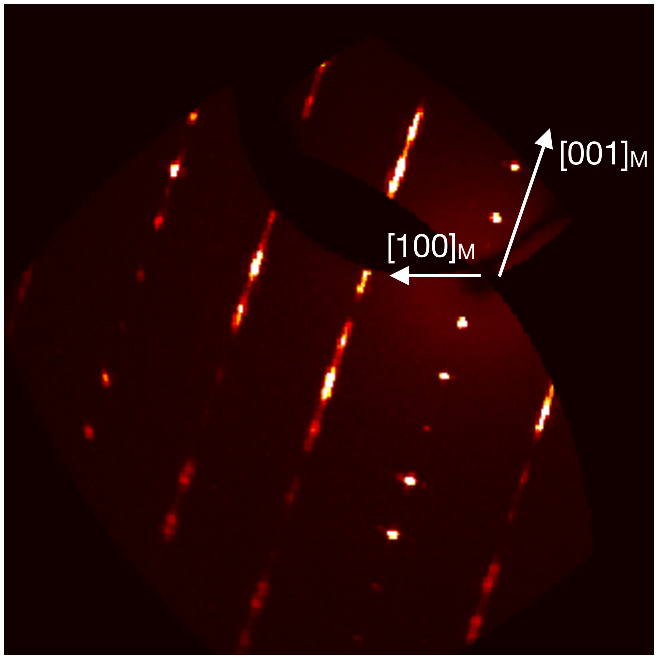


FIG. S1. Single crystal x-ray diffraction intensity in the $(H0L)_M$ plane, taken on a crystal cooled from 300 to 110 K. The transition into the $R\bar{3}$ phase is frustrated, resulting in diffuse scattering along $[001]_M$ similar to that seen for $\alpha$-$RuCl_3$ [2]. The peaks along $(00L)$ and $(\bar{6}0L)$, however, are unaffected.

$a_R$-axis lattice parameter obtained from data taken on cooling at POWGEN was determined from the position of $(300)_R$. In (b), the interlayer spacing was determined from the position of $(006)_R/(002)_M$. Generally, diffuse scattering makes obtaining the lattice parameters from Rietveld refinement difficult, but at 300 K (before the transition begins) the refinement value of $a = 5.9600(21)$ Å agrees with that obtained from $(300)_R$ ($a = 5.9592(3)$ Å), while the refined interlayer spacing $s = 5.7964(21)$ Å agrees with that obtained from $(002)_M$ ($s = 5.7954(3)$ Å.) The $a$ parameter shows an anomalous negative thermal expansion at low temperature. The interlayer spacing doesn't show a clear anomaly, though there may possibly be an anomalous downturn relative to the expected flattening-out of the dispersion as $T \to 0$ K (i.e., expected when the thermal expansion is due to phonon anharmonicity.) The lack of "flattening-out" of the interlayer spacing is, regardless, similar to the behavior of the $c$-axis lattice constant in $CrBr_3$ [3].

Single crystals also exhibit the negative thermal expansion, as we see from data taken on the triple-axis spectrometer SPINS (Fig. S3(c).) The $a$-axis lattice constant was determined from the position of $(\bar{1}, 2, 0)_R$ obtained via radial scans across the peak. The thermal history of the sample is shown in Fig. S3(d) by tracing the intensity of $(\bar{1}, 2, 0)_R$; following previous measurements at low temperature, the $(\bar{1}, 2, 0)_R$ intensity was measured on warming from 200 to 285 K, then cooling to 10 K.

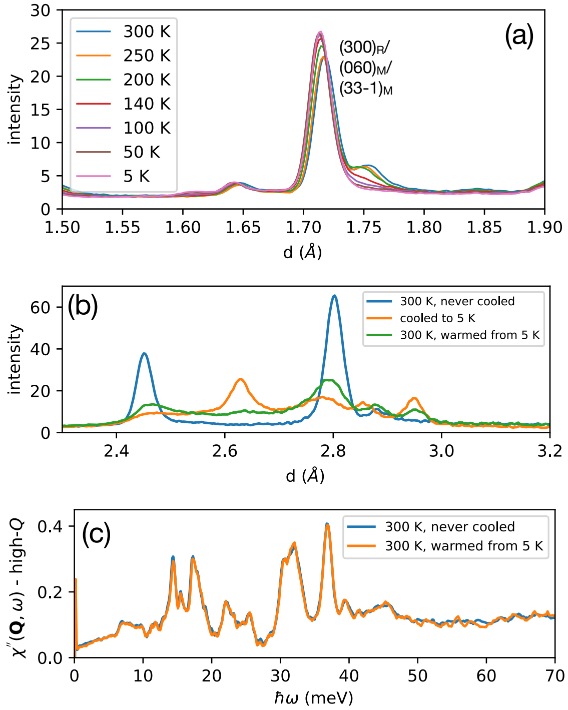


FIG. S2. (a) Elastic intensity in the vicinity of $(300)_R$, showing little change on cooling from 300 to 5 K. (b,c) Comparison of (b) elastic and (c) inelastic data taken at 300 K initially (i.e., before any cooling was done), after cooling to 5 K, and on warming back up to 300 K. All intensities in arbitrary units. Error bars omitted for clarity.

We see that the transition into the $C2/m$ phase is nearly complete by 285 K, and that most of the change back to $R\bar{3}$ occurs by 200 K. Thus, the transition in the single crystal was sharp, in contrast to the broad transition in our powder sample.

## EFFECT OF STACKING DISORDER ON INELASTIC SCATTERING

Because of the very weak structural and magnetic interactions between the $CrCl_3$ layers, we do not expect substantial changes in the inelastic data with stacking changes. It is instructive to compare data taken at 300 K before and after having cooled to 5 K. In Fig. S2(b), we see that most of the diffuse scattering present at 5 K in Fig. 1(b) of the main text (due to stacking disorder) is still present on warming back to 300 K, though the $(113)_R$ peak (at $d \sim 2.64$ Å) is diminished. Despite the stacking disorder, the inelastic intensity in Fig. S2(c) is almost unchanged.

The interlayer magnetic coupling is expected to be very weak, ∼0.003 meV for the simplified lattice discussed in Ref. [4]. We note, though, that the interlayer coupling is reported to increase tenfold for HT-type stack-

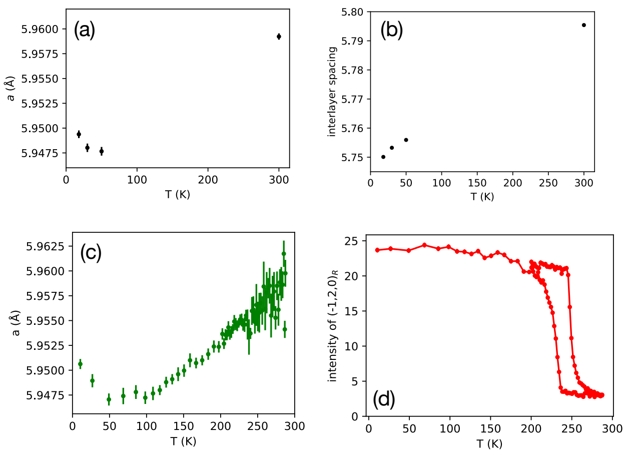


FIG. S3. (a) The $a$-axis lattice parameter and (b) interlayer spacing obtained from the $(300)_R$ and $(006)_R$ peak positions, respectively, from powder data taken on cooling at POWGEN. Errorbars in (b) are smaller than symbols. (c) The $a$-axis lattice constant obtained from the position of $(\bar{1},2,0)_R$, from data taken on a single crystal measured at SPINS. (d) The integrated intensity of $(\bar{1},2,0)_R$ (in arbitrary units), which indicates the degree to which the transition between the $C2/m$ and $R\bar{3}$ phases has proceeded. The data in (c,d) were taken on warming from 200 K (after previously at low temperatures) to 285 K, then cooling down to ∼10 K. The structural transition proceeded nearly ideally, though it was not complete after warming to 285 K, as shown from the intensity of $(\bar{1},2,0)_R$ in (d).

ing [5]. In Fig. S4, we show simulated powder-averaged $S_\perp(\mathbf{Q},\omega)$ for the $R\bar{3}$ structure without interlayer magnetic coupling, and the $R\bar{3}$ and $C2/m$ structures with a coupling $J_L = -0.04$ meV (i.e., larger than reported) between nearest-neighboring interlayer bonds. Only minor changes are seen between the three calculated intensities. With increasing $J_L$, there is a near-uniform shift upward of the dispersion, and a small amount of dispersion can be seen at the upper edge and near 0 meV. We note that the $C2/m$ structure has many more interlayer first-nearest neighbors (four, with lengths of 6.11 to 6.13 Å) than $R\bar{3}$ (one, of length 5.78 Å), so the same value of $J_L$ would lead to a more pronounced effect on $C2/m$ than $R\bar{3}$. We presume that the effect of stacking disorder would be intermediate between that of the $R\bar{3}$ and $C2/m$ structures and would, thus, be negligible.

## INSTRUMENT RESOLUTION

When computing the spin-wave intensities in Fig. 4(a), we convoluted the intensity with an energy resolution derived from formulas in Ref. [6], with the detector offset distribution $\delta R_2$ scaled to the width of the elastic peak; the overall intensity scale and backgrounds for the low- and high-$Q$ parts were adjusted manually to fit the data.

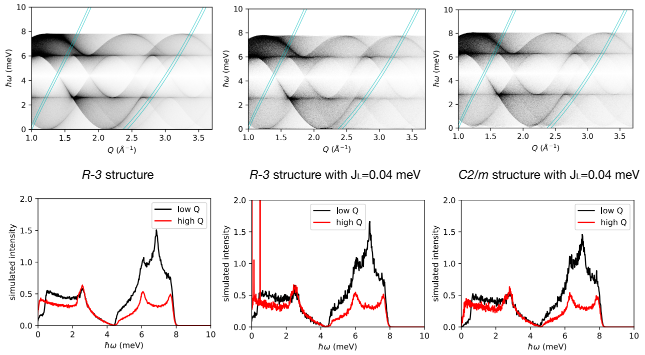


FIG. S4. (top) Simulated SpinW powder-averaged $S_\perp(\mathbf{Q},\omega)$ for the $R\bar{3}$ structures without interlayer interactions, and the $R\bar{3}$ and $C2/m$ structures with an interlayer coupling of $J_L = -0.04$ meV between nearest-neighboring interlayer bonds. (bottom) Simulated intensity along the low- and high-$Q$ trajectories for each of these cases.

## INTENSITY MAPS OF INELASTIC INTENSITY VS. TEMPERATURE

Fig. S5 shows intensity maps comprised of the low- and high-$Q$ inelastic data. These data are the same as those shown in Fig. 3(c-h) in the main text.

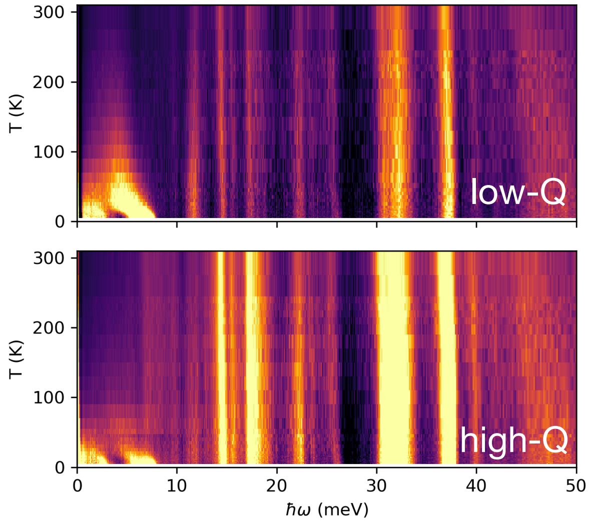


FIG. S5. Intensity maps of $\chi''$ $(Q,\omega)$ along the low- and high-$Q$ trajectories, plotted against temperature from many scans taken on cooling.

## RELAXATION OF LATTICE CONSTANTS AFTER DFT CALCULATIONS

In Table S1, we show the relaxed lattice constants obtained after DFT calculation (see Fig. 2(c) in the main

TABLE S1. Table of relaxed lattice constants obtained during DFT calculations for the $R\bar{3}$ structure with the specified magnetic ordering.

| | in-plane FM | in-plane AFM | inter-plane AFM |
|---|---|---|---|
| $a$ (Å) | 6.014 | 6.002 | 6.014 |
| $c$ (Å) | 17.283 | 17.339 | 17.295 |

text) for the in-plane FM, in-plane AFM, and inter-plane AFM order. As seen in the data, $a$ increases as we go toward FM in-plane spin correlation. The size of the change in the relaxed $a$ (0.2%) is about three times higher than the relative increase in $a$ in our data from 50 to 5 K ($\sim$0.06%), which is reasonable considering that, presumably, the spins in $CrCl_3$ start from being uncorrelated rather than anti-correlated.

## FITTING OF THE SPIN WAVE INTENSITY TO LINE SEGMENT FUNCTION

For the purpose of defining the location of the Dirac node energy or the corners of the upper branch hump, we fit our Bose-factor-corrected data to a function of connected line segments (plus a Gaussian near 2.5 meV for the low-$Q$ data.) The fits are shown in Fig. S6. The FWHM of the Gaussian was fixed at 0.538, the lowest value initially found from fitting that peak in the 5 to 7 K data. The fitted location of this peak in the high-$Q$ data at each temperature was used to fit the corresponding node in the low-$Q$ data. The positions of nodes are shown in Fig. S6(c,d), where the nodes were labeled from lowest to highest energy. The positions of the first and last nodes (#1 and #7) were fixed at 1 and 10 meV, respectively, but their intensities were allowed to vary.

## TEMPERATURE-DEPENDENCE OF OVERALL INTENSITY

As the temperature increases, we expect disorder to decrease the magnetic intensity faster at large $Q$ than at small $Q$ since small deviations of spin orientation have a disproportionate impact on the large-$Q$ neutron scattering intensity. We see this effect in Fig. S7, which shows the intensity summed within $1 \leq \hbar\omega \leq 10$ meV as a function of temperature for low- and high-$Q$. On warming, the low-$Q$ intensity has a plateau up to $\sim$17 K, then decreases, while the high-$Q$ intensity drops steeply even at 5 K and saturates more quickly.


[1] Bruno Morosin and Albert Narath, "X-Ray Diffraction and Nuclear Quadrupole Resonance Studies of Chromium Trichloride," The Journal of Chemical Physics **40**, 1958–1967 (1964).

[2] R. D. Johnson, S. C. Williams, A. A. Haghighirad, J. Singleton, V. Zapf, P. Manuel, I. I. Mazin, Y. Li, H. O. Jeschke, R. Valentí, and R. Coldea, "Monoclinic crystal structure of $\alpha$-$RuCl_3$ and the zigzag antiferromagnetic ground state," Physical Review B **92**, 235119 (2015).

[3] D. P. Kozlenko, O. N. Lis, S. E. Kichanov, E. V. Lukin, N. M. Belozerova, and B. N. Savenko, "Spin-induced negative thermal expansion and spin–phonon coupling in van der Waals material $CrBr_3$," npj Quantum Materials **6**, 1–5 (2021).

[4] Albert Narath and H. L. Davis, "Spin-Wave Analysis of the Sublattice Magnetization Behavior of Antiferromagnetic and Ferromagnetic $CrCl_3$," Physical Review **137**, A163–A178 (1965).

[5] Dahlia R. Klein, David MacNeill, Qian Song, Daniel T. Larson, Shiang Fang, Mingyu Xu, R. A. Ribeiro, P. C. Canfield, Efthimios Kaxiras, Riccardo Comin, and Pablo Jarillo-Herrero, "Enhancement of interlayer exchange in an ultrathin two-dimensional magnet," Nature Physics **15**, 1255–1260 (2019).

[6] Philip A. Seeger, Luke L. Daemen, and John Z. Larese, "Resolution of VISION, a crystal-analyzer spectrometer," Nuclear Instruments and Methods in Physics Research Section A: Accelerators, Spectrometers, Detectors and Associated Equipment **604**, 719–728 (2009).

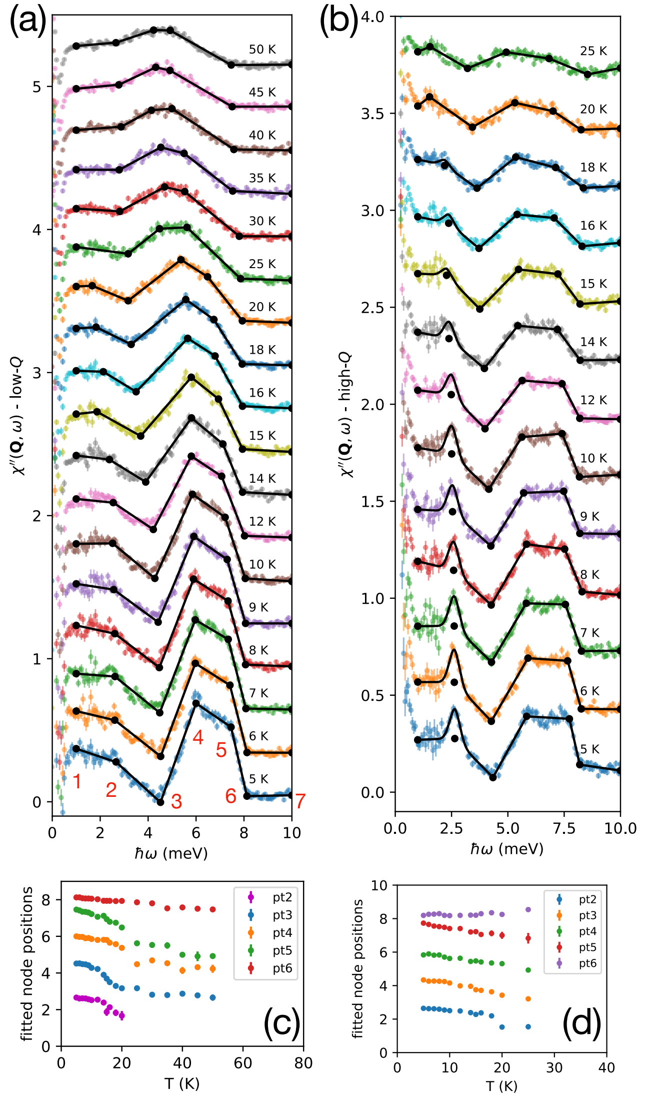


FIG. S6. (a,b) Data with the fitted function. The node positions are shown in (c,d). (a,c) are low-$Q$ data, and (b,d) are high-$Q$. Data in (a,b) are not smoothed.

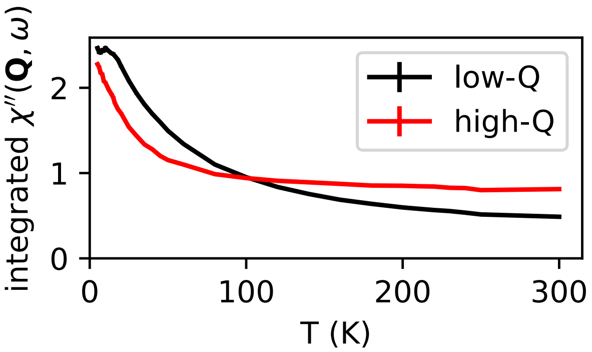


FIG. S7. $\chi''(\mathbf{Q},\omega)$ integrated within $1 \le \hbar\omega \le 10$ meV for the low- and high-$Q$ trajectories. Error bars are smaller than the linewidth.
